# Supplementary material for: Accelerated Convergence for Counterfactual Learning to Rank
Source: arXiv:2005.10615 source file (2020-05-21)
Supplement: Supplementary file 1 [file appendix.tex]

%!TEX root = ../sigir2020.tex

\section{Synthetic Learning Example}
\label{sec:appendix:synthetic}

In this appendix we describe the synthetic learning example used for Figure~\ref{fig:toy}.
We created this synthetic illustration to provide intuition why \OurMethod{} achieves a better convergence rate than scaling the loss or gradients with \ac{IPS} weights.

First, we generate a dataset of training instances by sampling $50$ two-dimensional samples:
\begin{flalign}
X = \left[ \begin{array}{ccc}
x_{1,1} & x_{1,2} \\
x_{2,1} & x_{2,2} \\
 \vdots & \vdots \\
 x_{50,1} & x_{50,2} 
\end{array} \right],
\end{flalign}
where each $x_{i,j} \sim \mathcal{N}(0, 1)$ and we denote with $x_i$ the $i$th row in $X$.
Next, we set $\bm{w}^* = [0.973, 1.144]$, and generate regression targets $y = \iprod*{X, \bm{w}^*}$.
Then, we randomly generate IPS weights for each data sample $x_{i}$: $p_i \sim \textit{Uniform}(0.05, 1.0)$.
Finally, we use the squared loss as our optimization objective:
\begin{equation}
R_{\textit{IPS}}(\bm{w}) = \frac{1}{50} \sum_{i=1}^{50} \frac{1}{p_i}\rbrackets*{\iprod*{x_{i}, \bm{w}} - y}^2
\end{equation}
